# Supplementary material for: Early processing of consonance and dissonance in human auditory cortex
Source: arXiv:1711.10991 source file (2017-11-30)
Supplement: Supplementary file 1 [file supplementaryMaterials.pdf]

# Supplementary materials to "Early processing of consonance and dissonance in human auditory cortex"

Alejandro Tabas*, Martin Andermann*, Valeria Sebold, Helmut Riedel
Emili Balaguer-Ballester+, & André Rupp+

## S1 Supplementary videos: model's dynamics

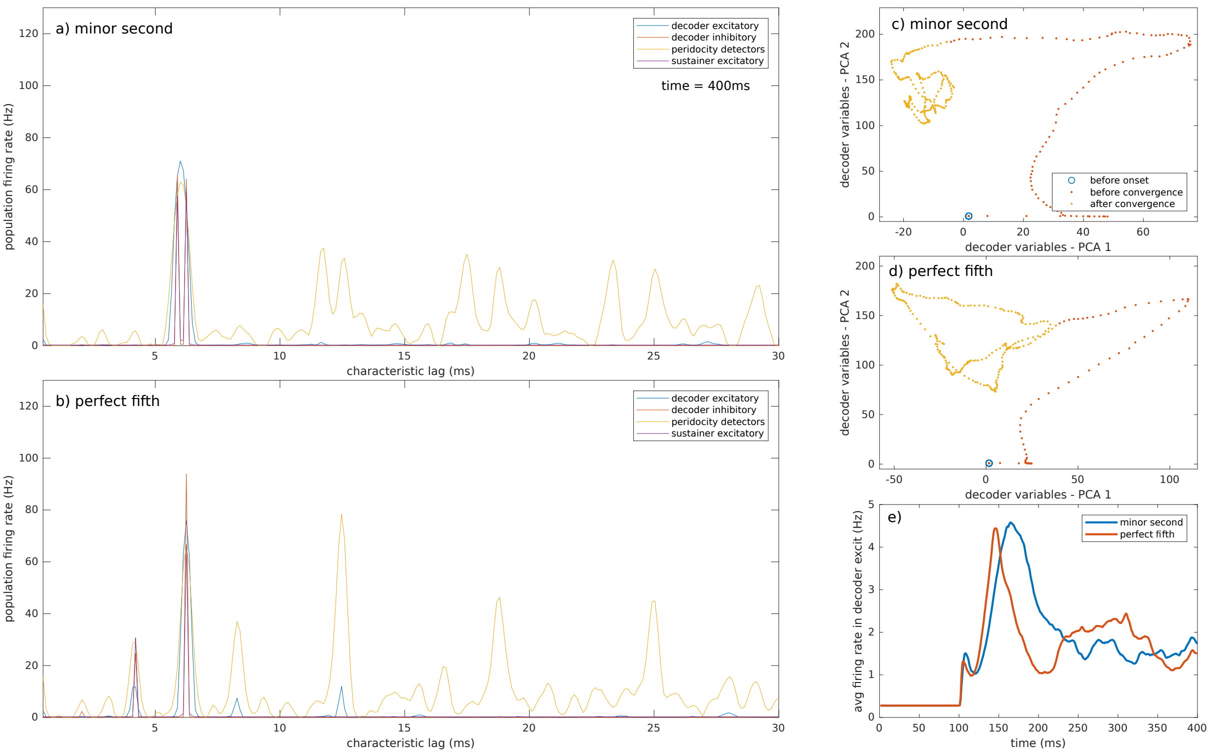


Video SS2: **Model dynamics during the processing of dyads.** a)–b) Instantaneous firing rate of the periodicity detectors (yellow), the ensembles in the decoder (excitatory blue, inhibitory red), and the excitatory ensemble in the sustainer (purple) for two IRN dyads: a minor second (a) and a perfect fifth (b). c)–d) 2-dimensional projection of the state variables of the decoder during pitch processing of a minor second (c) and a perfect fifth (d) dyad; see caption of Video S1 for more details. e) Aggregated excitatory activity in the decoder, monotonically related to the predicted elicited field in the generator of the POR, for each of the two dyads: the minor second (blue) and the perfect fifth (red). Note that the system converges earlier for the consonant dyad (the minor fifth), eliciting an earlier POR. Stimulus parameters were chosen as in Figures 4 and 5 in the main text.

## S2 Attractor dynamics of the model and pitch transitions

### S2.1 Decoder dynamics and the POR

The behavior of the decoding network can be characterized by a dynamic system with variables $\vec{x} = \{H_n^e, H_n^i, S_n^{\text{AMPA}}, S_n^{\text{NMDA}}, S_n^{\text{GABA}}\}^{n=1\ldots N}$. In absence of input drive, the system presents a single state of stable equilibrium around the origin $\vec{x} = \vec{x}_0 \simeq 0$.

Finite cortical inputs change the stability properties of the system. An excitatory cortical input moves the state of equilibrium towards a new attractor state termed here $\vec{x}_{\text{input}}$, where the excitatory

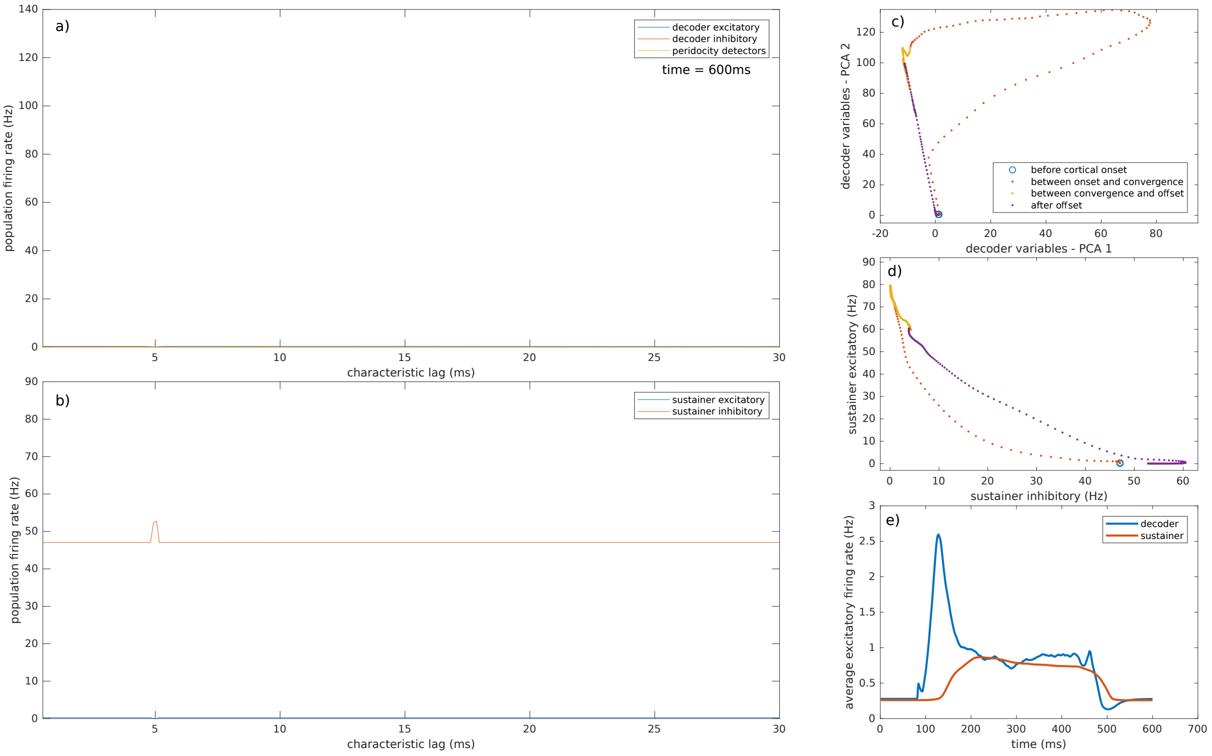


Video SS1: **Model dynamics during the processing of iterated rippled noise.** a) Instantaneous firing rate of the periodicity detectors (yellow) and the ensembles in the decoder (excitatory blue, inhibitory red). b) Instantaneous firing rate of the ensembles in the sustainer (excitatory blue, inhibitory red). c) 2-dimensional projection of the state variables of the decoder during pitch processing; projection axes were chosen as the two first principal components of the decoder's variables (i.e. the firing rates of the neural ensembles). Each dot represents the state of the system at a given instant $t$ with a step size of $\Delta t = 1\,\text{ms}$. Colors were used to characterize the different stages of the model dynamics: open blue circles represent the absence of input (points are too close to each other to be distinguished); red dots represent states within the time window spanning from the stimulus onset to the convergence of the model to a specific pitch value (at about 100 ms after sound onset); yellow dots represent states within temporal windows spanning from the convergence of the system to the tone's offset; purple dots show states in the time window corresponding to the the *relaxation dynamics*, spanning form the offset of the tone up to 200 ms after sound offset. d) Excitatory and inhibitory firing rate of the column characterizing the extracted pitch in the sustainer network. Note that the relaxation dynamics of the sustainer, corresponding to the trajectory of the system after offset (purple points), is much slower than the relaxation dynamics of the decoder (resembling the characteristic of the sustained field offset delay [1]). e) Aggregated excitatory activity in the decoder (blue) and the sustainer (red), monotonically related to the equivalent dipole moment of the elicited fields in each of the two networks. Stimulus parameters were chosen according to Krumbholz et al. [2]; i.e., same as in Figure 2 in the main text. Stimulus pitch was set to $f = 200\,\text{Hz}$ ($T = 5\,\text{ms}$).

populations represent the input activity (see Figure S1A). If the input presents a harmonic structure, the system converges to a second equilibrium state we termed $\vec{x}_1$ (see Figure S1A), characterized by excitatory and inhibitory activation at the column encoding the stimulus pitch.

We identify the POR as the neuromagnetic representation of this two-stage transition: the build up of the transient corresponds to the transition $\vec{x}_0 \to \vec{x}_{\text{input}}$; the POR peaks shortly after the onset of the decoding process, characterized by the transition $\vec{x}_{\text{input}} \to \vec{x}_1$ (see Figure S1A). This identification connects the POR latency with the time necessary to trigger the $\vec{x}_{\text{input}} \to \vec{x}_1$ transition; thus, the POR latency is informative of the convergence time in the decoding network (see also Figure S1).

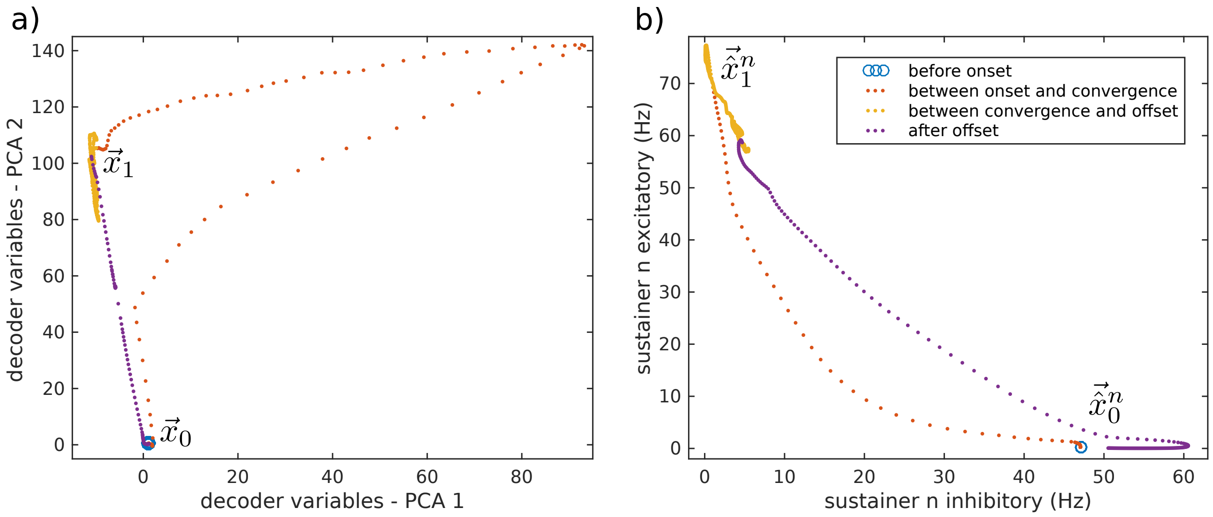


Figure S1: **Attractor dynamics underlying pitch processing.** a) View of a 2-dimensional projection of the state variables $\vec{x}$ during pitch processing (see caption in Video S1 for details). The trajectory in the reduced space reveals key aspects of the onset and relaxation dynamics; the transition from $\vec{x}_0$ to $\vec{x}_1$ characterizes the POR. b) View of the two dimensions of the subsystem characterizing the decoded pitch $n$ in the sustainer network. Note that the relaxation dynamics of the sustainer, corresponding to the transition from $\hat{\vec{x}}_1^n$ to $\hat{\vec{x}}_0^n$, are much slower than the relaxation dynamics of the decoder; resembling the sustained field offset delay [1].

## S2.2 Sustainer dynamics

The role of the sustainer network is to modulate the dynamic properties of the decoder in order to prevent the reversed transition $\vec{x}_1 \to \vec{x}_{\text{input}}$ and subsequent oscillations that are not observed in the recorded magnetic field responses.

The sustainer's dynamics is much simpler than the decoder dynamics; it consists of $N = 250$ uncoupled dynamical systems, one per column, with 5 variables each $\hat{x}^n = \left\{\hat{H}_n^e, \hat{H}_n^i, \hat{S}_n^{\text{AMPA}}, \hat{S}_n^{\text{NMDA}}, \hat{S}_n^{\text{GABA}}\right\}$. At rest, the decoder's independent variables lie in equilibrium states $\hat{\vec{x}}^n = \hat{\vec{x}}_0$ characterized by a strong activation in the inhibitory population and a null activation in the excitatory ensemble of each column $n$.

Combined excitatory and inhibitory input from the decoder network to a given subsystem $\hat{\vec{x}}^n$ causes inhibition to drop and excitation to rise, switching the ensembles of the column to a new state $\hat{\vec{x}}_1$ termed here *sustained state* (see Figure S1B). Top-down efferents from the sustainer then lock the selective dynamics of the layer decoder, strengthening the attractor properties of the state $\vec{x}_1$ and turning it to a state of stable equilibrium (see Figure S1b).

Subsequently, top-down efferents from the sustainer network lock to the pitch-selective dynamics of the decoder, strengthening the attractor properties of the decoder network state $\vec{x}_1$ and turning it to a robust stable equilibrium state (see Figure S1b).

When the cortical input is switched off (the behavior of the model under pitch changes is addressed in Figure S2), excitatory activity in the decoder drops, removing the excitatory input at the sustainer column $\hat{\vec{x}}^n$, which returns to its resting state $\hat{\vec{x}}_0$. As a result, the sustainer column stops modulating the dynamics of the decoder and the state $\vec{x}_1$ becomes, once again, unstable. Thus, the decoder state slowly relaxes back to the origin state $\vec{x}_0$.

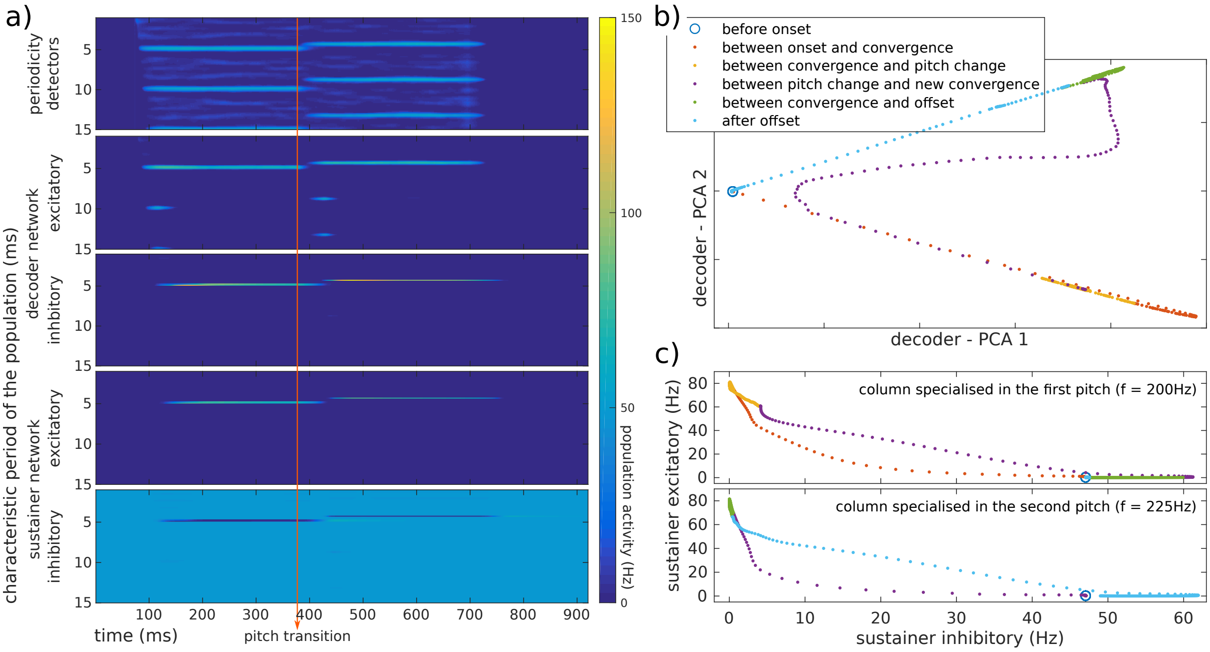


Figure S2: **System's reaction to pitch changes.** a) Response to pitch changes (see caption in Figure 2 in the Main Text for details). b)–c) Representation of the attractor dynamics of the model under pitch changes. Two colours were added to represent the new states in the system's evolution: purple now represents the dynamics from the second stimulus onset to the new state of convergence, defined here as the state achieved 100 ms after the onset; green represents states between 100 ms and the second stimulus' offset; and light blue represent the states during the relaxation dynamics after offset. The remaining colours are kept as in Video S1. Note that the transition from $\vec{x}_1$ to $\vec{x}_2$ elicits a new, second POR corresponding to the second stimulus. Stimuli were IRNs with the same specifications as in [2]; first tone had a fundamental frequency $f_0 = 200\,\text{Hz}$, second tone was two semitones higher than the first note, with $f_0 = 225\,\text{Hz}$. The pitch transition occurs 300 ms after the onset of the first tone (see arrow in the figure).

# S3 Additional predictions on the POR latency of simple IRNs

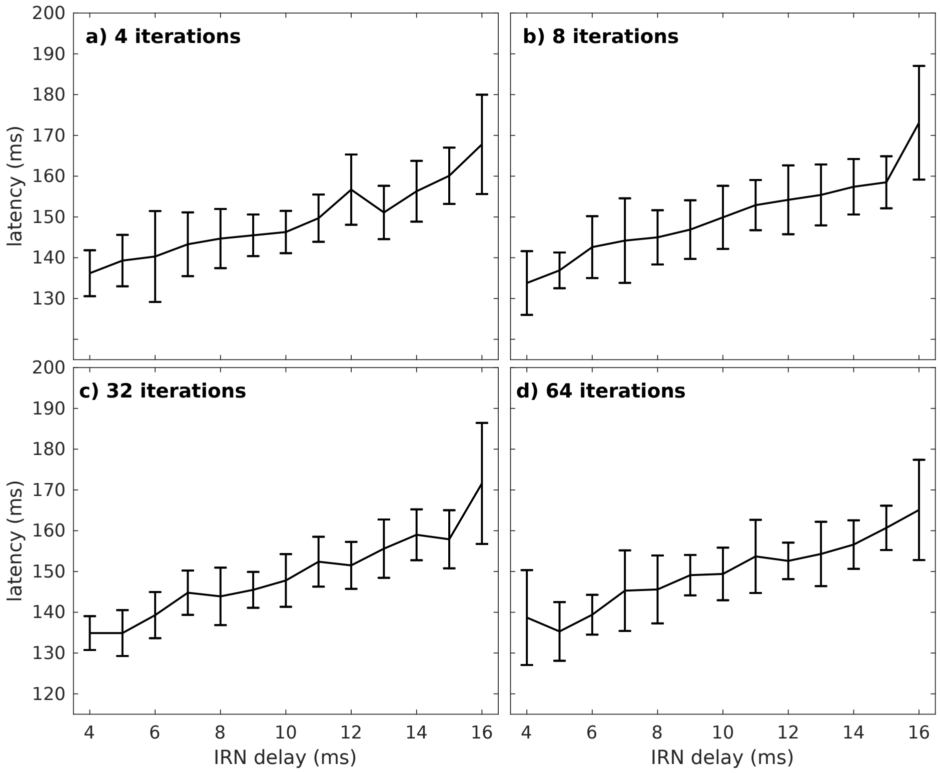


Figure S3: **Predicted latencies for additional families of IRNs.** Except for the number of iterations of the IRNs, simulation parameters were the same as in Figure 3a. Although experimental data is not available for these stimili, results depict a faithful replication of the trends reported in Figure 3a.

# S4 Additional predictions on the POR latency of dyads

# S5 Extrapolation of the POR predictions to other stimuli

Although our model successfully explained the morphology and latency of the POR elicited by stimuli based on iterated rippled noise, the extrapolation of these results to additional stimulus' types is limited by experimental constraints. Stimuli not based on IRN do not have an energy-matched counterpart; thus, their elicited POR cannot be disentangled from the rest of subcomponents on the N100 complex [4].

Here, we tackle this problem by expressing the N100 latency as an average between the latency of the POR and an hypothetical energy onset response (EOR). This simple model allows us to correct our POR predictions by assuming that the latency of the EOR is always 90 ms, that both transients have the same amplitude, and that their generators are equally distant from the N100 equivalent dipole. Corrected values are shown in Figures S5.

Despite the success of the simple model of the N100 introduced above, the generalization to further stimuli remains a challenge. For instance, harmonic complex tones elicit N100 transients with shorter peak latencies than the 90 ms latency assumed for the EOR above [6]. Future work should approach this issue by providing for a detailed model of the EOR and other (timbre-related) transients contributing to the N100 [7].

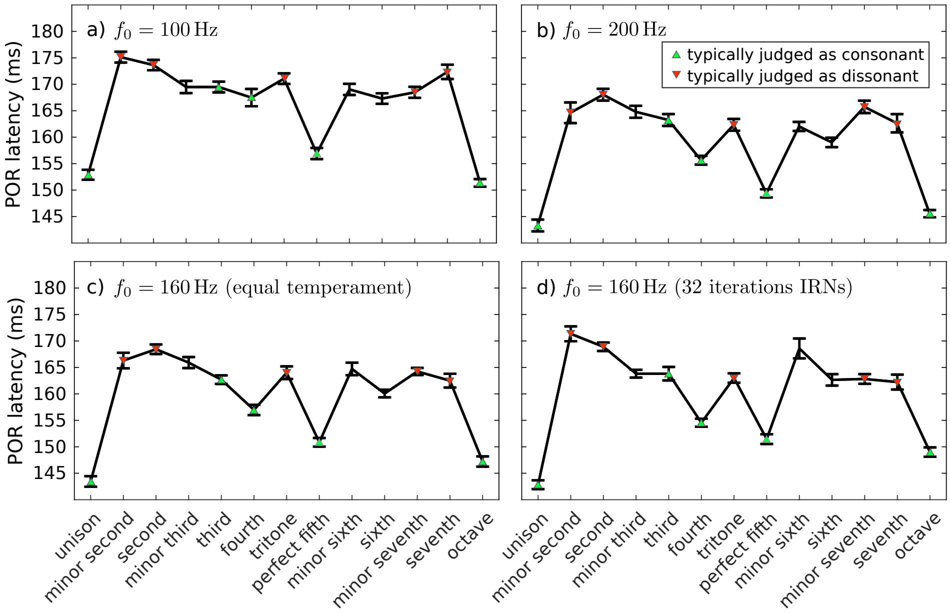


Figure S4: **Predicted latencies for additional families of dyads.** As in Figure 5k, strongly consonant dyads are represented with a green triangle, whilst strongly dissonant dyads are represented with a red triangle [3]. Dyad and experimental parameters were the same as in Figure 5k, with the following changes: a) lower-pitched dyads, with $f_0 = 100\,\mathrm{Hz}$ instead of $160\,\mathrm{Hz}$; b) higher-pitched dyads: $f_0 = 200\,\mathrm{Hz}$; c) *equal temperament* was used instead of the *just intonation* to calculate the chromatic scale; d) dyads were generated using IRNs with 32 rather than 8 iterations. These additional results faithfully reproduce the effect of consonance on latency reported in Figure 5. Moreover, panels a) and b) show that the latency differences due to pitch change are smaller than the latency differences induced by dissonance.

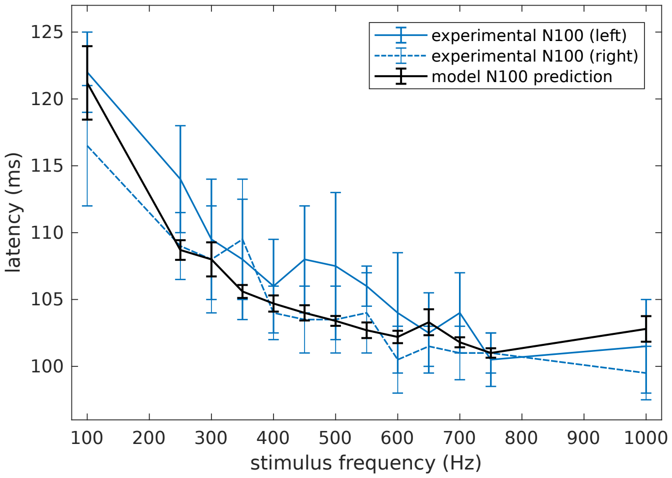


Figure S5: **Predicted latencies for pure tones.** a) Simulated N100 latency values (black error bars) in comparison with N100 latency observations (blue error bars); the two experimental curves correspond to latency values observed in the right and left hemispheres. Predictions were averaged along 5 runs of the model; error bars are standard deviations. Experimental data was taken from Roberts et al. [5], Fig 2.

## S6 Neural representations of the pitch value for additional stimuli

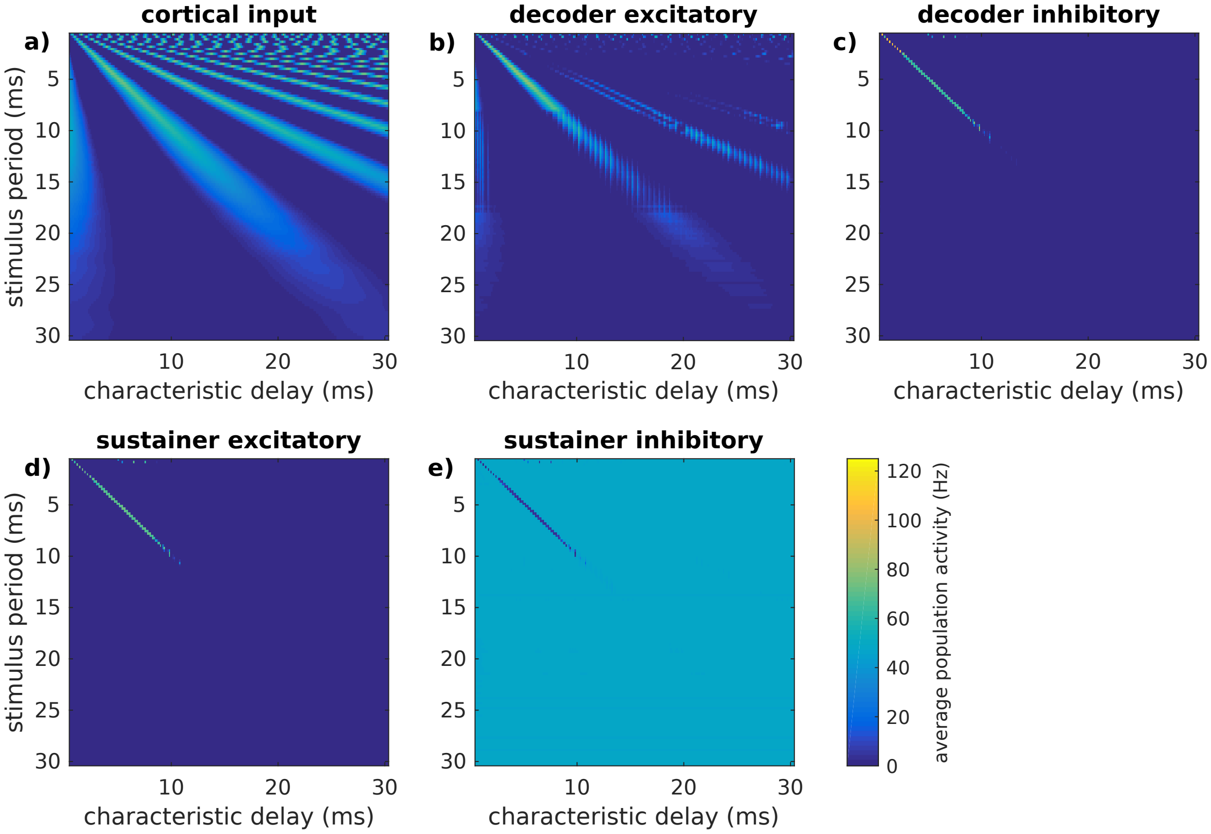


Figure S6: **Neural representation of the pitch value for pure tones.** Averaged model responses to pure tones at different stages of the model: (a) periodicity detectors, (b/c) excitatory/inhibitory ensembles in the decoder, (d/e) excitatory/inhibitory ensembles in the sustainer. The decay of the responses under $\sim 125$ (or $T \sim 8$) is due to the lower frequency limit of the peripheral model [8]. Figure was produced using the same methodology as in Figures 3C–3G (see Main Text for details).

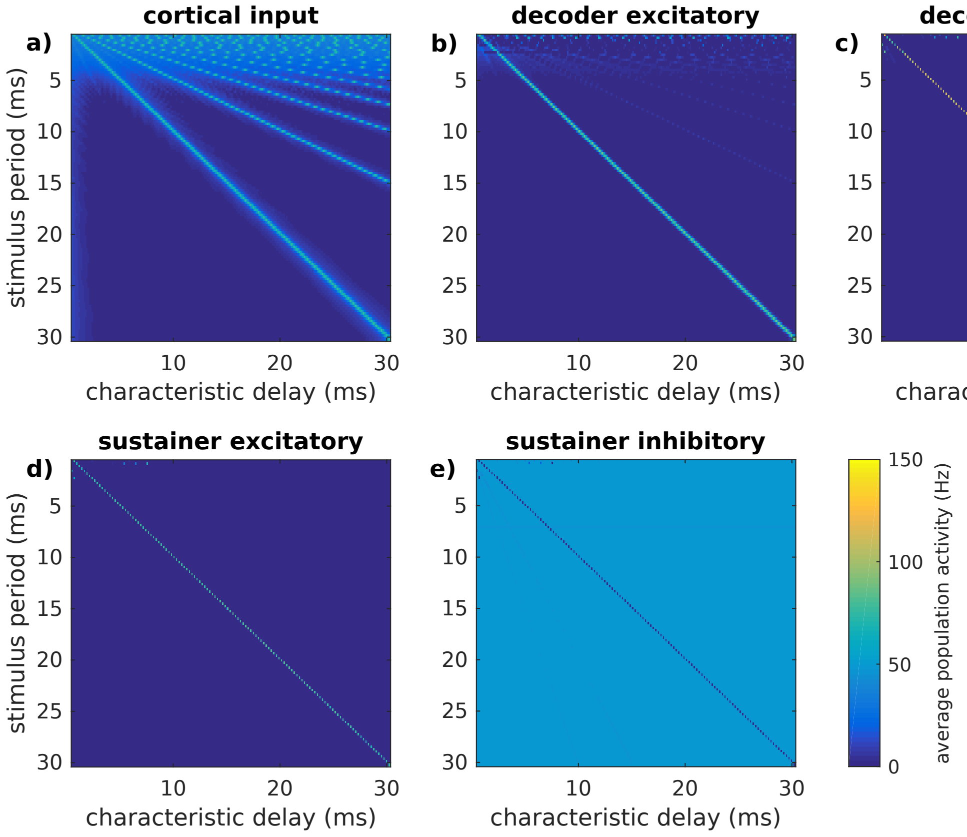


Figure S7: **Neural representation of the pitch value for click trains.** Click trains elicit the same pitch sensation as a sine wave with period $T$ equal to the interclick interval [9]. Perceptual results for click trains are shown in Figure S7; results are fully consistent with experimental observations [9]. Heat maps represent different stages/ensembles of the model (see caption of Figure S3). Click trains were generated as a train of Dirac deltas.

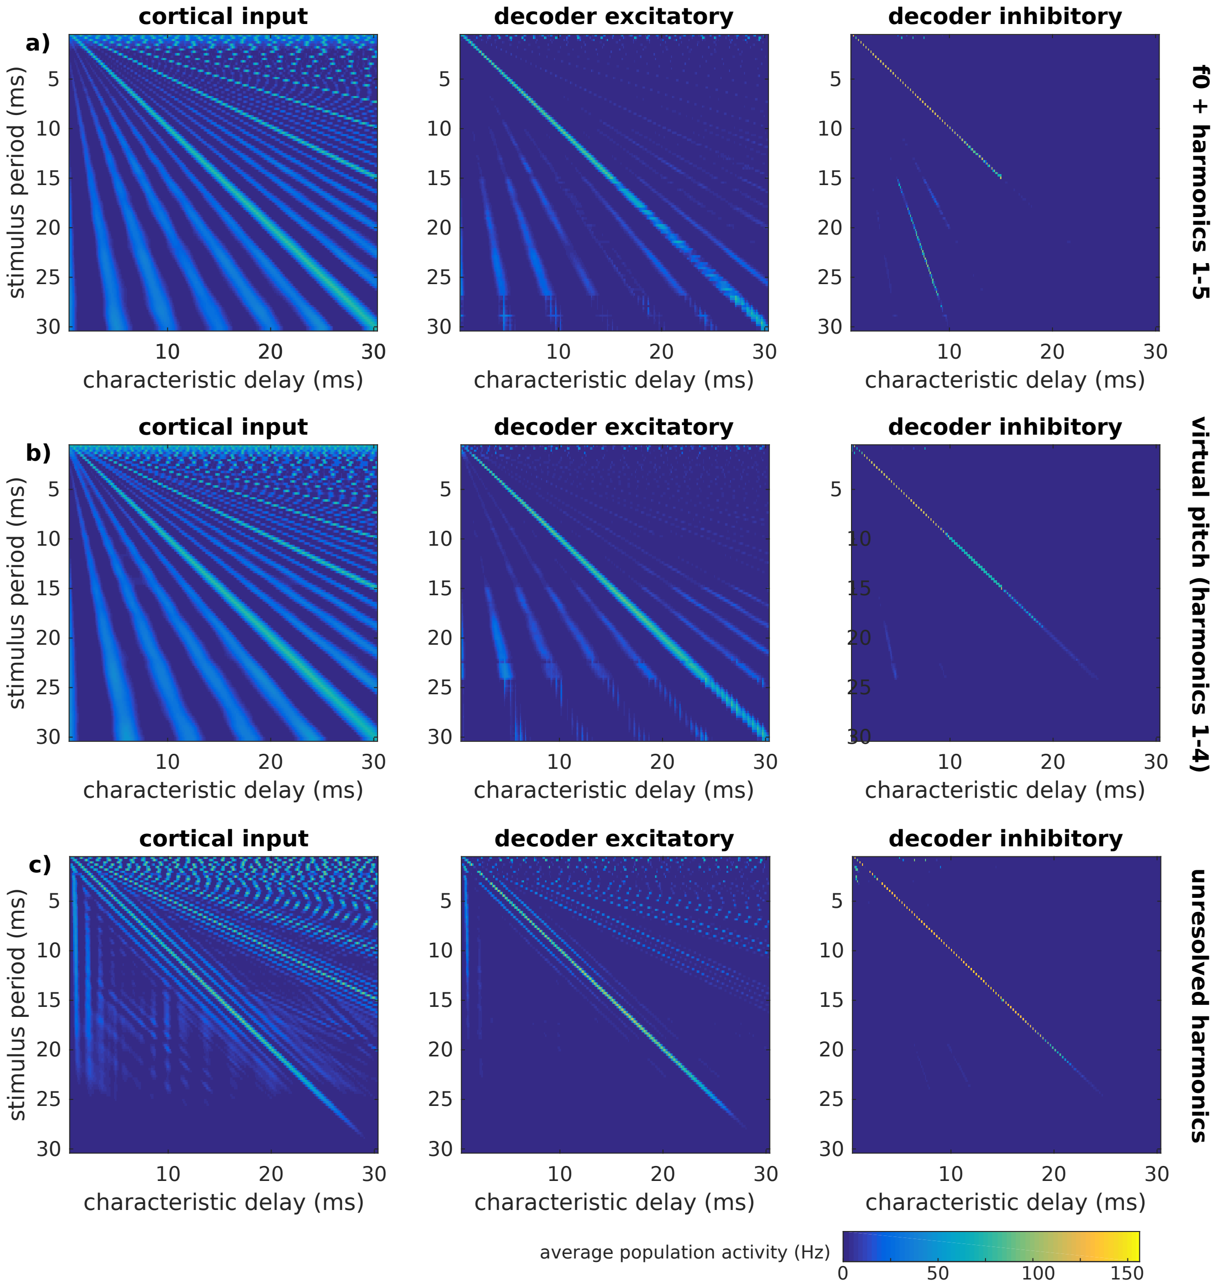


Figure S8: **Neural representation of the pitch value for harmonic complex tones.** HCTs elicit the same pitch percept as a sine wave with the frequency of the fundamental of the complex, even if the fundamental itself is not comprised in the complex; this phenomenon is known as *virtual pitch* [10]. The figure shows the responses of the model for: a) HCTs formed by the fundamental and the first 5 higher harmonics; b) HCTs with a missing fundamental (comprising only by the first four higher harmonics); c) HCTs with a missing fundamental comprising harmonics that are not independently resolved in the cochlea (tones were generated as harmonic complexes with harmonics 1 to 50, bandpass filtered between 3.2 kHz and 5 kHz). Note that, since the model uses several peaks of the harmonic series to extract the pitch value from the representation in the periodicity detectors, the perceptual range of the model is limited to periods $T < 15\,\mathrm{ms}$. Averaged responses in the sustainer populations are precisely correlated with the responses in the inhibitory ensembles in the decoder (see Figures S7 and S6; they are ommitted here for simplicity.

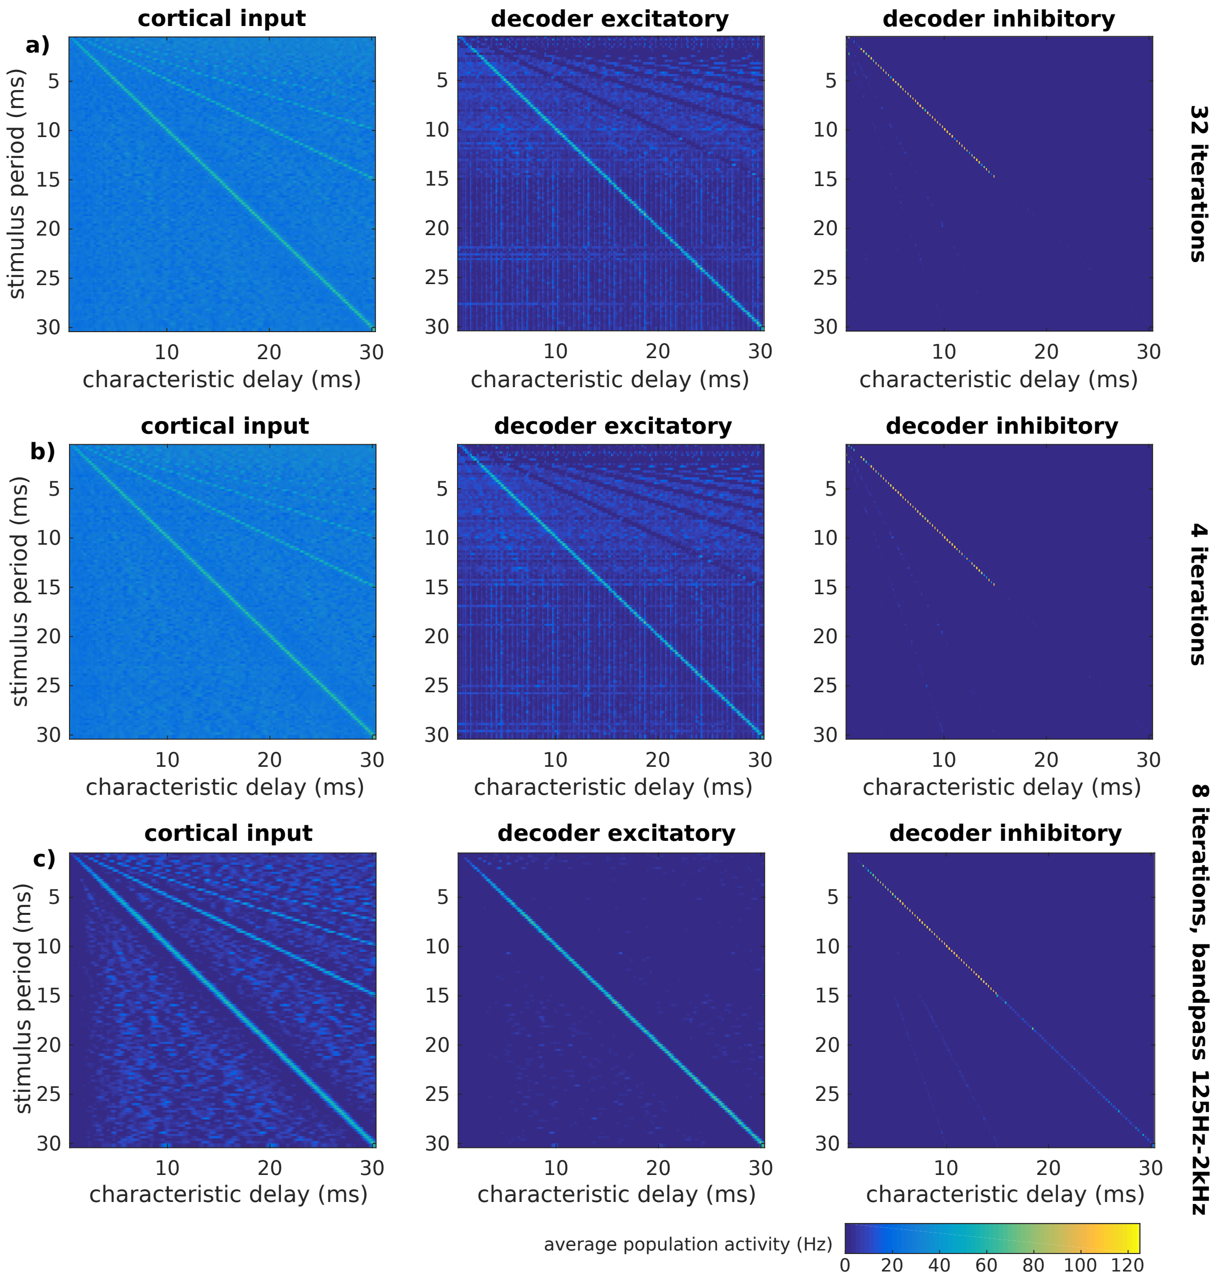


Figure S9: **Neural representation of the pitch value for additional iterated rippled noises.** The figure shows the perceptual responses for additional families of iterated rippled noises (IRN) with different parametrisations (see also Figure 3 in the Main Text): a) IRN with 32 iterations and no filtering; b) IRN with 4 iterations and no filtering; c) IRN with 8 iterations, bandpass filtered between 125 Hz and 2 kHz (this last parametrisation was chosen according to the IRN specifications of the dyads used in the experiments in the Main Text). Notice again the lack of responses out of the perceptual range of the model (i.e., for $T > 15\,\mathrm{ms}$).

# S7 Supplementary Methods: Regularisation of the input to the decoder network

The output of the coincidence detectors basef on the summary autocorrelation function (SACF) [11–13] at each characteristic period $A_n(t)$ is regularised $A_n(t) \to \check{A}_n(t)$ through a four steps procedure that reduces the dependence of stimulus intensity levels and minimises strong signal-to-noise variations with timbre.

In the first step, $A_n(t)$ is low-passed by a $\tau = 20\,\mathrm{ms}$ leaky-integrator that reflects the degradation of phase-locked activity over 50 Hz in auditory cortex [14]. The low-passed $A_n(t)$ is then normalised by dividing the overall signal by the low-passed summary self-correlation of the auditory nerve activity [15]. A fixed baseline $b_0 = 0.35$ is then subtracted from the overall function. Baseline was chosen such that a white noise stimulus elicits no activation, in agreement with fMRI studies that reported pitch-selective activation in inferior colliculus [16, 17].

Last, the normalized baseline-corrected $A_n(t)$ is rescaled to firing rate units (Hz) by a constant factor $A_0 = 75\,\mathrm{Hz}/(1 - b_0)$ that yields typical input activation peak values of $\sim 60\,\mathrm{Hz}$, in agreement with previous cortical models of perceptual integration [18]. Average activation in the regularised SACF associated to dyads was around half of the size of the average activation elicited by single IRNs (with the only exception of the unison, which was essentially a single IRN). Thus, in order to preserver the same $\sim 60\,\mathrm{Hz}$ peak activation also in dyads we used a doubled rescaling factor ($A_0^{\mathrm{dyads}} = 2\,A_0$).

## References


[1] A. Gutschalk, R. D. Patterson, A. Rupp, S. Uppenkamp, and M. Scherg, "Sustained magnetic fields reveal separate sites for sound level and temporal regularity in human auditory cortex.," *NeuroImage*, vol. 15, pp. 207–16, jan 2002.

[2] K. Krumbholz, R. D. Patterson, A. Seither-Preisler, C. Lammertmann, and B. Lütkenhöner, "Neuromagnetic evidence for a pitch processing center in Heschl's gyrus," *Cerebral Cortex*, vol. 13, no. 7, pp. 765–772, 2003.

[3] H. L. F. von Helmholtz, *Die Lehre von den Tonempfindungen als physiologische Grundlage für die Theorie der Musik.* Braunschweig: Vieweg, 1863.

[4] R. Näätänen and T. Picton, "The N1 wave of the human electric and magnetic response to sound: a review and an analysis of the component structure.," *Psychophysiology*, vol. 24, no. 4, pp. 375–425, 1987.

[5] T. P. Roberts, P. Ferrari, S. M. Stufflebeam, and D. Poeppel, "Latency of the auditory evoked neuromagnetic field components: stimulus dependence and insights toward perception," *Journal of Clinical Neurophysiology*, vol. 17, no. 2, pp. 114–29, 2000.

[6] A. Seither-Preisler, R. Patterson, K. Krumbholz, S. Seither, and B. Lütkenhöner, "Evidence of pitch processing in the N100m component of the auditory evoked field.," *Hearing Research*, vol. 213, pp. 88–98, mar 2006.

[7] M. Andermann, R. D. Patterson, C. Vogt, L. Winterstetter, and A. Rupp, "Neuromagnetic correlates of voice pitch, vowel type, and speaker size in auditory cortex.," *NeuroImage*, vol. 158, pp. 79–89, 2017.

[8] M. S. A. Zilany and L. H. Carney, "Power-Law Dynamics in an Auditory-Nerve Model Can Account for Neural Adaptation to Sound-Level Statistics," *Journal of Neuroscience*, vol. 30, pp. 10380–10390, aug 2010.

[9] W. T. Catton, "Tone Sensation produced by Repetitive Trains of Auditory 'Click' Stimuli," *Nature*, vol. 168, pp. 882–882, nov 1951.

[10] E. Terhardt, "Pitch, consonance, and harmony," *The Journal of the Acoustical Society of America*, vol. 55, no. 5, pp. 1061–1069, 1974.

[11] R. Meddis and L. O'Mard, "A unitary model of pitch perception.," *The Journal of the Acoustical Society of America*, vol. 102, pp. 1811–1820, sep 1997.

[12] R. Meddis and L. P. O'Mard, "Virtual pitch in a computational physiological model," *The Journal of the Acoustical Society of America*, vol. 120, no. 6, p. 3861, 2006.

[13] E. Balaguer-Ballester, S. L. Denham, and R. Meddis, "A cascade autocorrelation model of pitch perception.," *The Journal of the Acoustical Society of America*, vol. 124, pp. 2186–95, oct 2008.

[14] J. F. Brugge, K. V. Nourski, H. Oya, R. a. Reale, H. Kawasaki, M. Steinschneider, and M. a. Howard, "Coding of repetitive transients by auditory cortex on Heschl's gyrus.," *Journal of neurophysiology*, vol. 102, pp. 2358–74, oct 2009.

[15] A. de Cheveigné, "Pitch Perception Models," in *Pitch: Neural Coding and Perception* (C. J. Plack, R. R. Fay, A. J. Oxenham, and A. N. Popper, eds.), ch. 6, pp. 169–233, Springer New York, 2005.

[16] T. D. Griffiths, S. Uppenkamp, I. Johnsrude, O. Josephs, and R. D. Patterson, "Encoding of the temporal regularity of sound in the human brainstem.," *Nature Neuroscience*, vol. 4, pp. 633–7, jun 2001.

[17] H. Penagos, J. R. Melcher, and A. J. Oxenham, "A neural representation of pitch salience in nonprimary human auditory cortex revealed with functional magnetic resonance imaging.," *The Journal of Neuroscience*, vol. 24, pp. 6810–5, jul 2004.

[18] K.-F. Wong and X.-J. Wang, "A recurrent network mechanism of time integration in perceptual decisions.," *The Journal of Neuroscience*, vol. 26, no. 4, pp. 1314–1328, 2006.
